# Supplementary material for: Making expert processes visible: how and why theorists use assumptions and analogies in their research
Source: arXiv:2204.13652 ancillary file (2022-11-10)
Supplement: Supplementary file 1 [file Theorist_Interview_Protocol.pdf]

## Theoretical Physicist Interview Protocol

- Intro
  - Introducing ourselves (who we are, schools, REU program)
  - We are currently gathering data for a physics education research project about the cognitive processes and lives of theoretical physicists. We are hoping to understand the primary skills that a theoretical physicist uses in their research and how these are different from what students are learning. Additionally, we hope to make theoretical physics accessible to students, as well as the public.
  - We are going to ask you a series of questions about your work. Please answer to the best of your ability and feel free to include technical terms if they are important to your answer. We would like to keep the interview within the hour, but please feel free to discuss your work as you deem fit. As mentioned in the email, we are going to be recording this interview so we can refer back to it.
- Basic info questions:
  - Okay, so now we're going to start by asking a few basic info questions to get to know you a bit better.
  - What are your degrees in (B.A./B.S, PhD)?
  - What is your job/profession?
  - What field(s) do you do research in?
  - Would you consider yourself purely a theorist? If no, what percentage of the work that you do is theory?
  - We're trying to honor and acknowledge the researchers' experience from different backgrounds. Could I ask you about your age, gender and ethnicity, and/or any other identities you have you'd like to share?
- Applied Cognitive Task Analysis/Critical Decision Method questions:
  - Now we're going to take an overview of a project that you have recently completed.
  - Task Diagram
    - Can you think of a research project that you worked on, preferably somewhat recently, and has been completed?
    - Can you please give a couple minute overview of the project, so we have some background?
    - Think about the process you took to complete this project, start to finish. Can you split this into 10 stages or so? These don't have to be detailed steps, just a general process.
  - Knowledge Audit
    - Next, we would like to get a more in depth look into the cognitive tasks that occurred during the research projects.
    - Where did the research goal originate?
      - Was this a standard way for a project to originate?

- What information made you decide to go forward with this project, in other words, how did you know this project was doable and significant?
  - Did you ask for feedback from others?
  - Were you already familiar with the literature and current research on the topic, or did you have to do background research?
  - Are there any “red flags” for a research project that make you decide not to go through with it? Has this ever happened after you’ve already started?
  - At any point before starting the research, did you have an idea of what you would conclude?
  - How did you receive funding for this project? Is this typical for your research projects?
- Once you decided you were going to do this project, where did you start?
  - How did you decide to start here?
- At what points in your project did you have to make significant decisions, for instance decisions about the direction or scope of the project?
  - What information allowed you to make these decisions?
  - What experience was necessary to make these decisions?
  - Did your goals and objectives change at any point during the project?
- How much of your progress was made by using work directly from textbooks/papers versus applying/modifying ideas that others have come up with versus completely coming up with your own ideas?
- Was any part of your work done through collaboration?
  - How did you meet your collaborators? Are they theorists/experimentalists?
  - What was the nature of the collaboration?
  - How do you and the collaborator benefit from by collaborating?
  - When you collaborate with others do you give an overview of the math, or do you tell your mathematical steps in detail?
- Do you have any postdocs or grad students?
  - Did they work on the same project as you or different ones? Is this typical?
  - How do you work with them to decide what tasks they will work on?
- At any point during this project, did you face any difficulties or challenges?
  - What kinds of errors were made?
  - Why did you get stuck?
  - How did you move past these challenges?
  - Did you learn anything that you can use moving forward to avoid similar issues?
- How did you know when you had completed this project?

- At any point did you think you had finished and then realized you hadn't?
    - Were your results what you expected them to be?
    - Do you have an idea of any future directions, given your findings?
  - What methods have you used to present your findings?
    - Why did you choose to present your work this way? (Or why didn't you choose to do other things I guess)
- Questions about Math
  - We would like to take a closer look into the nature of the math that was used in the stages you laid out in your task diagram.
  - In which of the stages discussed previously did math play a significant/important role?
  - Questions to be asked in each stage requiring math:
    - *Within this stage of the project where you [fill in name here], could you please describe how mathematics was used?*
      - *What were some of the specific mathematical steps that you took during this project?*
      - *How did you know to do those things you just discussed?*
      - *How did you make the decision to take this mathematical step or approach?*
    - *When you used math (looking at each time individually), in what form or representation was it used? For instance, software, symbolic math, numbers, diagrams, geometric relationships, data, etc.*
      - *Why that representation? What does it accomplish? How long does it take to use?*
    - *What sort of math products or outcomes were generated during this stage?*
      - *For example, an answer to a question, figures, equations, derivations, etc.*
    - *Where did you learn the technical skills used in this stage?*
  - Were there any important parts of your process that we haven't discussed?
- General/day-to-day questions (if time)
  - Finally, we are going to ask you some more general questions about your career and day-to-day research life.
  - What does a day-in-the-life look like for you/general schedule?
    - What is your meeting schedule (how often do they occur)? One-on-one meetings? Group meetings?
    - How much of your time is spent doing research versus other things?
  - What is the motivation, what gratification do you get on short-term and long-term work? New ideas? Reaching some long-term goal?
    - How has this changed throughout your career?
  - How would you describe your relationship with experimental physics?

- How has your “job” changed as computational power has increased over the years?
- What are some of the things that make you good at what you do? These might be qualities that someone new to the field doesn’t have yet.
  - What advice do you have for someone entering or wanting to enter theoretical physics? (Consider parts of your education, or steps you took, that prepared you well for this career)
- What do you think is the reputation of theoretical physics according to undergraduates? Do you think this is an accurate assessment?
  - Are there any other things you would want undergraduate students to know about what it means to do theoretical physics?
  - What do you think the reputation is according to the public?
- Conclusion/Thank You
  - Thank you so much for your time!
